# Supplementary material for: Photo-induced charge-transfer renormalization in NiO
Source: arXiv:2305.10145 ancillary file (2024-05-24)
Supplement: Supplementary file 1 [file Lojewski_supplement_arxiv1.pdf]

# Photo-induced charge-transfer renormalization in NiO: Supplementary material

Tobias Lojewski,<sup>1</sup> Denis Golež,<sup>2,3</sup> Katharina Ollefs,<sup>1</sup> Loïc Le Guyader,<sup>4</sup> Lea Spieker,<sup>1</sup> Nico Rothenbach,<sup>1</sup> Robin Y. Engel,<sup>5</sup> Piter S. Miedema,<sup>5</sup> Martin Beye,<sup>5</sup> Gheorghe S. Chiuzbaian,<sup>6</sup> Robert Carley,<sup>4</sup> Rafael Gort,<sup>4</sup> Benjamin E. Van Kuiken,<sup>4</sup> Giuseppe Mercurio,<sup>4</sup> Justina Schlappa,<sup>4</sup> Alexander Yaroslavltssev,<sup>4,7</sup> Andreas Scherz,<sup>4</sup> Florian Döring,<sup>8</sup> Christian David,<sup>8</sup> Heiko Wende,<sup>1</sup> Uwe Bovensiepen,<sup>1,9</sup> Martin Eckstein,<sup>10</sup> Philipp Werner,<sup>11</sup> and Andrea Eschenlohr<sup>1</sup>

<sup>1</sup>*Faculty of Physics and Center for Nanointegration Duisburg-Essen (CENIDE),  
University of Duisburg-Essen, Lotharstr. 1, 47057 Duisburg, Germany*

<sup>2</sup>*Jozef Stefan Institute, Jamova 39, 1000 Ljubljana, Slovenia*

<sup>3</sup>*Faculty of Mathematics and Physics, University of Ljubljana, Jadranska 19, 1000 Ljubljana, Slovenia*

<sup>4</sup>*European XFEL, Holzkoppel 4, 22869 Schenefeld, Germany*

<sup>5</sup>*Deutsches Elektronen-Synchrotron DESY, Notkestr. 85, 22607 Hamburg, Germany*

<sup>6</sup>*Sorbonne Université, CNRS, Laboratoire de Chimie Physique - Matière et Rayonnement, 75005 Paris, France*

<sup>7</sup>*Department of Physics and Astronomy, Uppsala University, 75120 Uppsala, Sweden*

<sup>8</sup>*Paul Scherrer Institut, Forschungsstr. 111, 5232 Villigen PSI, Switzerland*

<sup>9</sup>*Institute for Solid State Physics, The University of Tokyo, Kashiwa, Chiba 277-8581, Japan*

<sup>10</sup>*I. Institute of Theoretical Physics, University of Hamburg, 20355 Hamburg, Germany*

<sup>11</sup>*Department of Physics, University of Fribourg, 1700 Fribourg, Switzerland*

(Dated: May 17, 2023)

## DATA PROCESSING

This section of the supplementary material details the steps taken in analysing the experimental data. The absorption spectra are measured in transmission geometry in accordance with the employed beam-splitting off-axis zone plate setup [1] and are evaluated using the dedicated Spectroscopy and Coherent Scattering (SCS) Instrument toolbox [2]. From the transmitted signal, X-ray absorption spectroscopy (XAS) is calculated as the negative logarithm of the transmitted signal divided by the reference signal, where the flat-field and non-linearity corrections [2] are also incorporated. Likewise, the pump-induced change is derived by taking the negative logarithm of the fraction between the excited spectrum and the ground-state spectrum.

### Correction of background

The evaluated Ni  $L_{23}$  edge absorption spectra show a background in the form of an offset between the ground state and excited spectrum, which we attribute to the zone plate setup. In addition, the two spectra slightly deviate over the measured energy range, as the offset increases slightly with increasing photon energy. The background is corrected using two identical linear functions of opposite signs, which are constructed from the difference between the spectra in the pre- and post-edge region. Thus the ground state and excited spectra coincide in the pre- and post-edge regions after the correction, as shown in Fig. 1(b) of the main paper. After the background correction, the spectra are normalised such that the mean value in the pre-edge corresponds to 0 while the

mean value of the post-edge corresponds to 1, as shown in Fig. 1(b). The induced changes, as determined by the SCS toolbox [2], are also corrected with the linear background function and then scaled according to the normalisation of the spectra to ensure continued agreement between the two. In order to also normalise the delay scans, an average normalisation factor is determined from all the absorption spectra for each pump laser fluence, which is then used to scale the induced changes.

For the Oxygen  $K$  edge, the background takes a more complicated form that cannot be captured with a linear approximation. The background still shows an offset like the Ni  $L_{23}$  edge spectra, however, the spectra appear to diverge with a quadratic background. From some of the delay scans that we measured, we can determine that in addition to the pre- and post-edge regions, there are no pump-induced changes from 533 eV to 534 eV and from 548 eV to 550 eV as well. Using these regions as a reference, we can correct the background in the same manner as we did at the Ni  $L_{23}$  edges, however, now we use a quadratic function rather than a linear one. Following the background correction, the spectra are also normalised such that the mean value in the pre-edge region corresponds to 0 while the mean value of the post-edge corresponds to 1.

### Analysis of pump-induced changes

In order to analyse the experimental spectra, we aim to extract the modifications of the ground-state spectrum that would reproduce the excited-state spectrum. A rigid energy shift and a broadening are considered as individual modifications for the Nickel  $L_{23}$  edges and Oxygen  $K$  edge. We calculate an Akima spline of the ground-

state spectrum and include the energy shift by shifting the energy axis by an amount  $\Delta E$  relative to the original ground-state spectrum. The broadening is incorporated by convoluting this Akima spline with a Gaussian with the full width at half maximum (FWHM)  $\omega$ . By calculating the difference between the Akima spline and ground-state spectrum, we get a modelled induced change that we can optimise with these two parameters. This modelled pump-induced change is optimised for the Nickel  $L_{23}$  edges over the whole energy range (845-875 eV). For the Oxygen  $K$  edge, we optimise the model at the measured induced changes of the first peak between 525 eV and 532.5 eV. This is done since using the whole energy range leads to an overall worse agreement of the model, because the second and fourth fine structure peaks show some additional modifications that are not described with an energy shift and broadening. By fixing one of the parameters to be zero, we can show that both modifications are necessary to describe the measured induced changes at the Nickel  $L_{23}$  edges and Oxygen  $K$  edge.

As the calculated spectra shown in Fig. 3(a) of the main paper show a narrowing with increased photodoping, the model used to describe the pump-induced changes in the experimental data is not applicable to the calculations, in particular for larger photodoping values. Instead, in order to determine the energy shift and narrowing, a Voigt profile is fitted to the calculated data. The energy shift is then determined as the difference between the central peak positions, whereas the broadening/narrowing is determined as the difference between the overall FWHM. For smaller photodoping, both the same modelling as for the experimental data as well as the fit of a Voigt profile can be applied, which show an overall excellent agreement for the determined energy shift. The determined values for the broadening/narrowing do deviate, however, although the trends are still similar.

For the visual representation of the delay scans, an additional binning is applied. The initial binning of the delay scans is chosen such that a data point is measured every 100 fs to ensure that even the fastest response can be resolved. However, this time resolution is only necessary immediately before and following the laser excitation, as the induced change is long-lived. In order to keep the figures neater, the scans are binned so that four data points are consolidated into one new data point in the areas far off the laser excitation, as shown in Fig. S1. The line added in the figures Fig. S1 and Fig. 2(a) of the main paper is meant as a guide for the eye and is obtained by fitting a response function [3]:

$$A_0 + \Theta(t - t_0) \left( A_1 \cdot \left[ 1 - e^{\frac{-(t-t_0)}{\tau_1}} \right] \cdot \left[ e^{\frac{-(t-t_0)}{\tau_2}} \right] + A_2 \cdot \left[ 1 - e^{\frac{-(t-t_0)}{\tau_2}} \right] \right) \quad (S1)$$

This function is convoluted with a Gaussian function

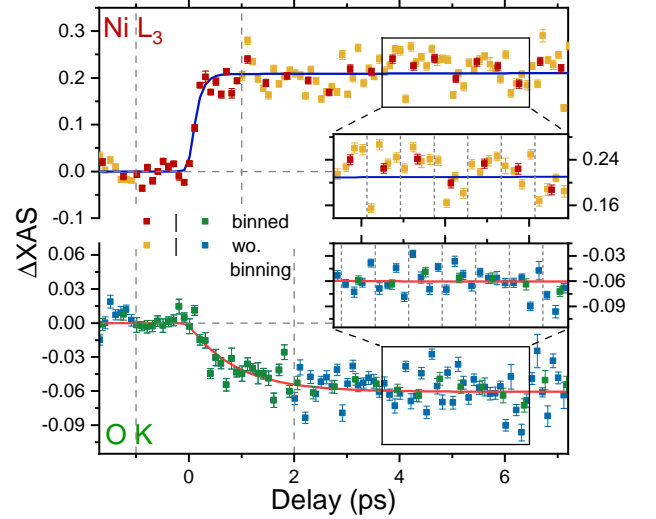

FIG. S1: Time-dependence of  $\Delta XAS$  at the Ni  $L_3$  (top) and O  $K$  (bottom) edge, for the excited charge carrier density of  $dn = 4.7\%$  and different binning at longer delays.

with the FWHM  $\Gamma_{tr} = 80$  fs to consider the time resolution. For the shown delay scans, the second time constant  $\tau_2$  converges towards infinity if left unconstrained, as no recovery is apparent. As such, this time constant was fixed for the final fit to reduce the number of free parameters and increase fit quality. The data is fitted to the original data and shows that there are no deviations resulting from the additional binning.

## CALCULATION OF EXCITATION DENSITY

During the experiment, we measured the laser fluence to be  $0.8 \text{ mJ/cm}^2$  and  $4.0 \text{ mJ/cm}^2$  corresponding to the number of incoming photons ( $n_{ph}^{in}$ ) with  $1.07 \cdot 10^{15} \text{ photons/cm}^2$  and  $5.36 \cdot 10^{15} \text{ photons/cm}^2$ , respectively. In order to calculate the photoexcitation for comparison with theory, we first calculate the number of absorbed photons ( $n_{ph}^{abs}$ ) using Beer-Lambert's law:

$$n_{ph}^{abs} = n_{ph}^{in} - n_{ph}^{in} \cdot e^{-\mu(E) \cdot d} \quad (S2)$$

Here  $\mu(E)$  is the absorption coefficient and is set as  $503000 \text{ 1/cm}$  according to [4], while  $d$  is the film thickness in cm. From this, we calculate the excitation density as:  $\frac{p_{e-} \cdot n_{ph}^{abs}}{d} \text{ e}^-/\text{cm}^3$ , with  $p_{e-}$  being the probability of a photo-excitation, which we assume to be 0.55. However, values between 0.1 and 1 are also possible. This value is then normalised to the unit cell value of NiO, where we assume the lattice constant to be  $4.2 \text{ \AA}$ , resulting in the photodoping values  $dn$  of  $0.9 \%$  ( $0.8 \text{ mJ/cm}^2$ ) and  $4.7 \%$  ( $4.0 \text{ mJ/cm}^2$ ) with an estimated error of  $82 \%$ .

## THEORETICAL MODELS AND METHODS

A full simulation of time-resolved XAS in a microscopic model for NiO, which would include on equal footing the multi-orbital character of the Ni  $d$  shell, the ligand orbitals, and a self-consistent description of the screening of local interaction parameters such as the Hubbard  $U$ , would be computationally very challenging. We therefore present two separate model calculations to analyze the different mechanisms at play: (i) In the first part, we compute time-resolved XAS within a standard model of charge-transfer insulators [5], namely the Emery or  $d$ - $p$  model [6] with strong correlations on the transition metal  $d$  orbitals and weaker correlations on the oxygen orbitals. Within the time-dependent GW+EDMFT framework [7, 8], this model allows us to study how the excitonic resonance in the XAS signal is modified in response to the redistribution of electrons between the  $p$  and  $d$  orbitals, and the modified screening of local interactions after the photo-excitation. (ii) In the second part, we focus on the two active  $e_g$  orbitals in NiO and describe them using a two-band Hubbard model, to understand how local many-body multiplet effects manifest themselves in the time-resolved XAS signal after the photoexcitation.

### Emery model

*Model* — The three band Emery model includes one correlated orbital ( $d$ ) and two ligand orbitals ( $p_x$  and  $p_y$ ) per unit cell in a cubic lattice. The  $d$  orbital is located at the sites of the lattice, while the  $p_x$  and  $p_y$  orbitals are located on the  $x$  and  $y$  bonds between the  $d$  sites, respectively. The Hamiltonian is given by

$$\begin{aligned} H_{dp} &= H_e + H_{\text{kin}} + H_{\text{int}}, \\ H_e &= \epsilon_d \sum_i n_{id} + \epsilon_p \sum_i (n_{ip_x} + n_{ip_y}), \\ H_{\text{kin}} &= \sum_{\langle i,j \rangle, \sigma, (\alpha, \beta)} (t_{ij}^{\alpha\beta} + \vec{E} \cdot \vec{D}_{ij}^{\alpha\beta}) e^{-\varphi_{ij}} c_{i\alpha\sigma}^\dagger c_{j\beta\sigma}, \\ H_{\text{int}} &= U_{dd} \sum_i n_{id\uparrow} n_{id\downarrow} + U_{pd} \sum_i n_{id} N_{i,p}, \end{aligned} \quad (\text{S3})$$

where  $c_{i\alpha\sigma}$  is the annihilation operator for unit cell  $i$  and orbital  $\alpha \in \{d, p_x, p_y\}$  with spin  $\sigma$ , and  $n_{i,\alpha,\sigma}$  is the corresponding density operator, and  $n_{i,\alpha} = \sum_\sigma n_{i,\alpha,\sigma}$ . In the interaction term  $H_{\text{int}}$ ,  $N_{i,p}$  measures the total occupation on the four  $p$  orbitals which connect to the  $d$ -site in unit cell  $i$  (in total two  $p_x$  and two  $p_y$  orbitals). The energy splitting  $\Delta = \epsilon_p - \epsilon_d$  is chosen such that the oxygen orbitals in the atomic limit are completely filled. The hopping matrix  $t_{ij}^{\alpha\beta}$  takes a nonzero value  $t^{dp}$  for hopping between nearest neighbor  $d$  and  $p_x$ ,  $p_y$  orbitals, and  $t^{pp}$  for hopping between the  $p_x$  and  $p_y$

orbitals;  $-t_{ii}^{\alpha\alpha} = \mu$  is the chemical potential. We excite the system by an electric field pulse, described by a homogeneous vector potential  $\vec{A}(t)$  and an electric field  $\vec{E}(t) = -\partial_t \vec{A}(t)$ . The vector potential enters into the kinetic part of the Hamiltonian via the Peierls phase  $\varphi_{ij} = e/\hbar \int_{R_i}^{R_j} d\vec{r} \vec{A}(t)$ , while the electric field couples via a dipolar matrix element  $\vec{D}_{ij}^{\alpha\beta}$  to the interorbital transitions [8]. The specific shape of the electric field used is  $E(t) = E_0 \exp^{-4.6(t-t_0)^2/t_0^2} \sin(\omega(t-t_0))$ , where  $E_0$  is the amplitude of the field and  $t_0$  is chosen such that the pulse includes four oscillations. We adjust the interaction and hopping parameters by comparing the equilibrium spectral function with LDA+DMFT results for NiO [9], leading to  $U_{dd} = 7.5$  eV,  $t^{dp} = 0.37$  eV,  $t^{dd} = -0.3$  eV,  $U_{pd} = 1.0$  eV and  $\Delta = -4.0$  eV. The dipolar matrix element was chosen as  $D = 0.3e_0a$ , where  $a$  is the lattice distance and  $e_0$  is the electron charge. We solve the dynamics after the photoexcitation in the valence space using the time-resolved GW+EDMFT method, which treats the strong correlation and screening effects on the same footing, see Refs. 7 and 8 for details. In the simulations, we adjust the amplitude of the electric field  $E_0$  such that the pulse produces a certain photo-excitation density  $dn$ . The latter is measured as a change of the density of the  $d$  orbital  $dn = n_d(t_{\text{fin}}) - n_d(t=0)$ , where  $t_{\text{fin}}$  is the final propagation time.

For numerical reasons, we restrict the modelling to a two-dimensional lattice and the paramagnetic phase. We do not expect that changing from the two-dimensional to the three-dimensional case would lead to qualitative differences, as the dominant effects are mainly local. The introduction of antiferromagnetic correlations can be expected to enhance the gap reduction after the photoexcitation and contribute to a larger renormalization of the main excitonic resonance [10].

*Evaluation of the XAS signal* — Within DMFT-based simulations, the calculation of the XAS signal is handled in a postprocessing step (see Ref. 11 for a detailed description of the formalism in the time-resolved case): We start from the DMFT impurity model, which describes one  $d$  orbital embedded in the lattice. (For GW+EDMFT simulations, the impurity model includes both the fermionic environment, and the dynamically screened local interactions [8].) To this model we explicitly add the core level, so that the impurity Hamiltonian is extended by the terms

$$H_{\text{post}} = H_c + H_{\text{dip}} + H_{cd} + H_{cp}.$$

Here the first term  $H_c$  describes a single core level,

$$H_c = \epsilon_c n_c,$$

where  $\epsilon_c$  is the core level energy,  $n_c$  is the density operator for the core hole, and  $H_{\text{dip}}$  describes the dipolar transitions between the core and valence orbitals. Because the X-ray energies  $\omega_{\text{in}}$  (of the order of 1 keV) are

much larger than the energies in the valence band (of the order of 1 eV), we treat the dipolar transitions from the core level to the  $d$  orbital within the rotating wave approximation, as detailed in Ref. 11. In this case, the X-ray transition energies are determined relative to a given reference, which can be the core level energy  $|\epsilon_c|$ , or a constant shift thereof. Throughout this paper we choose the energy reference as the position of the main excitonic line in the unperturbed system, denoted by  $|E_c|$ . A core-hole typically decays within a few femtoseconds, mainly due to Auger processes [12]. This decay implies an extrinsic broadening of the XAS transition lines, in addition to intrinsic line-shape effects that are related to the valence band final states. In the DMFT formalism for time-resolved XAS [11], a near-exponential decay of the core hole is implemented by coupling the core level to an electron reservoir with a wide Gaussian density of states. We use a bandwidth  $W/t_{dp} = 40.0$  for the bath, and choose the coupling strength to fix a lifetime  $\Gamma = 0.05\text{fs}^{-1}$ .

The interaction between a core hole and the valence electrons on the  $d$  site is described by a local density-density interaction with strength  $U_{cd}$  given by  $H_{cd} = U_{cd}(n_c - 2)n_d$ , where the shift of the core density is chosen such that the term vanishes for systems without core hole. The value of the core-valence interaction is comparable to the Coulomb repulsion on the  $d$  orbital [13] and we have chosen them to be equal,  $U_{cd} = 7.5\text{eV} = U_{dd}$ . We have checked that the photoinduced changes are robust with respect to variations of the core-valence interaction  $U_{cd}$ , up to a rigid shift of the XAS peaks. Similarly, we include the interaction between the core hole and the valence electrons on the  $p$  orbitals. We assume an interaction term  $H_{cp} = U_{cp}(n_c - 2)N_p$ , where  $N_p$  measures the total occupation on the four  $p$  orbitals adjacent to the probe site, analogous to the interaction  $U_{pd}$  in Hamiltonian (S3). Within the DMFT framework, this non-local interaction enters the impurity model as a Hartree shift of the  $c$  orbital,  $H_{cp}^{HF} = U_{cp}(n_c - 2)\langle N_p(t) \rangle$ , where  $\langle N_p(t) \rangle = 2\langle n_{px} + n_{py} \rangle$  is the occupation of the  $p$  orbitals obtained from the self-consistent GW+EDMFT simulation. (The factor two accounts for the fact that each correlated site has two neighboring  $p_x$  and two  $p_y$  orbitals; by symmetry,  $\langle n_{px} \rangle = \langle n_{py} \rangle$ ).

### Two-band Hubbard model

The dynamics of the active  $e_g$  orbitals in NiO is modelled using the two-band Hubbard model Hamiltonian

$$H = -t_{\text{hop}} \sum_{i,\alpha \in \{1,2\}} (c_{i\alpha}^\dagger c_{i\alpha} - \mu) + \sum_{i,\alpha} U n_{i\alpha\uparrow} n_{i\alpha\downarrow} + \sum_{i,\sigma} [(U - 2J_H) n_{i1\sigma} n_{i2\bar{\sigma}} + (U - 3J_H) n_{i1\sigma} n_{i2\sigma}], \quad (\text{S4})$$

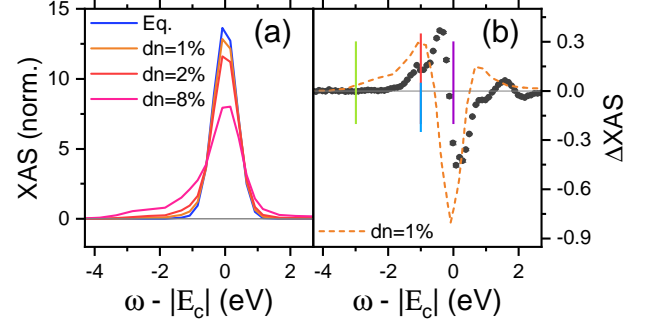

FIG. S2: (a) Calculated Ni  $L_3$  XAS in equilibrium (blue line) and evaluated within the two-band Hubbard model for increasing  $dn$  as indicated. (b) Measured Ni  $L_3$   $\Delta$ XAS at  $\Delta t = 0.25$  ps (symbols) with vertical lines marking the positions of the atomic transitions (from left to right)  $2s \rightarrow 3d$ ,  $2l \rightarrow 3d$  (degenerate with  $1d \rightarrow 2h$ ) and  $2h \rightarrow 3d$  (degenerate with  $1d \rightarrow 2l$ ). The dashed line corresponds to the model calculation with  $dn = 1\%$ . We have fixed the parameters of the model to  $U = U_{cd} = 7.5$  eV,  $J_H = 1$  eV,  $\beta = 5$  eV $^{-1}$ .

where  $i$  ( $\alpha$ ) is the site (orbital) index,  $t_{\text{hop}}$  is the hopping integral,  $U$  is the Coulomb repulsion and  $J_H$  is the Hund interaction.

We solve this model in the atomic limit and using DMFT on the Bethe lattice with bandwidth  $W = 4$  eV, see also the analysis in Ref. 11. In contrast to GW+EDMFT, the DMFT calculation cannot capture any bandgap renormalization, but it can describe the photo-generation of local many-body multiplets, like Hund excitations.

In the atomic limit, the main X-ray excitonic transition corresponds to  $2h \rightarrow 3d$  and its energy is given by  $\omega = E(3d) - E(2h) = (U + J_H)/2 - U_{cd} - \epsilon_c$ . Other transitions from excited states populated by the pump excitation include

1.  $2l \rightarrow 3d$  whose energy is given by  $\omega = E(3d) - E(2l) = (U - J_H)/2 - U_{cd} - \epsilon_c$ . This state corresponds to the main side peak discussed in the main text. As the difference to the main excitonic resonance is the spin configuration and not the charge configuration, the energy separation between these states is independent of the core-valence interaction  $U_{cd}$ .
2.  $2s \rightarrow 3d$  whose energy is given by  $\omega = E(3d) - E(2s) = (U - 5J_H)/2 - U_{cd} - \epsilon_c$ . The energy difference of this transition to the main excitonic peak is independent of the core-valence interaction  $U_{cd}$ .
3.  $1d \rightarrow 2h$  whose energy is given by  $\omega = E(2h) - E(1d) = -(U + J_H)/2 - \epsilon_c$ . This state has a different charge configuration than the main excitonic

resonance and the difference between the two will depend on the core-valence interaction  $U_{cd}$  as presented in Fig. 4 of the main manuscript.

4.  $1_d \rightarrow 2_l$  whose energy is given by  $\omega = E(2_l) - E(1_d) = (-U + J_H)/2.0 - \epsilon_c$ . The energy difference with respect to the main excitonic peak depends on the core-valence interaction  $U_{cd}$ .

The atomic limit analysis is consistent with the full DMFT simulation of the photoexcited system, as shown in Fig. S2(a) for  $dn = 1\%$  photodoping. Here, the system is excited by a hopping modulation pulse with an envelope  $a_{\text{pump}} \exp[-(t - t_{\text{pump}})^4]$  centered at time  $t_{\text{pump}} = 1.5 \text{ eV}^{-1}$  and with amplitude  $a_{\text{pump}} = 0.15 \text{ eV}$ . (In equilibrium, the hopping parameter  $t_{\text{hop}}^*$  in the Bethe lattice calculation is related to the bandwidth by  $W = 4t_{\text{hop}}^*$ .) The XAS probe pulse has an envelope  $a_{\text{probe}} \exp[-(t - t_{\text{probe}})^2/8]$  centered at  $t_{\text{probe}} = 6.5 \text{ eV}^{-1}$  and amplitude  $a_{\text{probe}} = 0.01 \text{ eV}$ . We use here a setup with explicit core level at energy  $-20 \text{ eV}$ , as described in Ref [11].

These DMFT simulations show that the photoinduced transition with the highest weight is  $2_l \rightarrow 3_d$ , although there also appears a pronounced shoulder corresponding to the transition  $2_s \rightarrow 3_d$  for higher photodopings. The DMFT and atomic limit analysis agree with the position of the experimental side peak, as shown in Fig. S2(b), but these calculations cannot capture the combined effect of the bandgap renormalization and the side peak appearance. Describing both effects would require an extension of the GW+EDMFT formalism to a two-orbital problem on the  $d$  site, which is an important future challenge. Our results nevertheless suggest that with future experimental advances in time-resolved XAS it may become possible to measure the occupations of local many-body states, since these are directly reflected in the heights of the photo-induced resonances.

---

[1] F. Döring, B. Rösner, M. Langer, A. Kubec, A. Kleibert, J. Raabe, C. A. F. Vaz, M. Lebugle, and C. David, *Optica* **7**, 1007 (2020).

[2] L. Le Guyader, A. Eschenlohr, M. Beye, W. Schlottter, F. Döring, C. Carinan, D. Hickin, N. Agarwal, C. Boeglin, U. Bovensiepen, J. Buck, R. Carley, A. Castoldi, A. D'Elia, J.-T. Delitz, W. Ehsan, R. Engel, F. Erdinger, H. Fangohr, P. Fischer, C. Fiorini, A. Föhlisch, L. Gelisio, M. Gensch, N. Gerasimova, R. Gort, K. Hansen, S. Hauf, M. Izquierdo, E. Jal, E. Kamil, S. Karabekyan, T. Kluyver, T. Laarmann, T. Lojewski, D. Lomidze, S. Maffessanti, T. Mamrybayev, A. Marcelli, L. Mercadier, G. Mercurio, P. S. Miedema, K. Ollefs, K. Rossnagel, B. Rösner, N. Rothenbach, A. Samartsev, J. Schlappa, K. Setoodehnia, G. Sorin Chiuzbaian, L. Spieker, C. Stamm, F. Stellato, S. Techert, M. Teichmann, M. Turcato, B. Van Kuiken, H. Wende, A. Yaroslavl'tsev, J. Zhu, S. Molodtsov, C. David, M. Porro, and A. Scherz, *Journal of Synchrotron Radiation* **30**, 284 (2023).

[3] N. Del Fatti, C. Voisin, M. Achermand, S. Tzortzakakis, D. Christofilos, and F. Vallée, *Phys. Rev. B* **61**, 16956 (2000).

[4] R. Newman and R. M. Chrenko, *Phys. Rev.* **114**, 1507 (1959).

[5] J. Zaanen, C. Westra, and G. A. Sawatzky, *Phys. Rev. B* **33**, 8060 (1986).

[6] V. Emery, *Phys. Rev. Lett.* **58**, 2794 (1987).

[7] D. Golež, L. Boehnke, M. Eckstein, and P. Werner, *Phys. Rev. B* **100**, 041111 (2019).

[8] D. Golež, M. Eckstein, and P. Werner, *Phys. Rev. B* **100**, 235117 (2019).

[9] J. Kuneš, V. I. Anisimov, A. V. Lukoyanov, and D. Vollhardt, *Phys. Rev. B* **75**, 165115 (2007).

[10] X. Wang, R. Y. Engel, I. Vaskivskyi, D. Turenne, V. Shokeen, A. Yaroslavl'tsev, O. Grånäs, R. Knut, J. O. Schunck, S. Dziarzhytski, *et al.*, *Faraday Discussions* **237**, 300 (2022).

[11] P. Werner, D. Golež, and M. Eckstein, *Phys. Rev. B* **106**, 165106 (2022).

[12] F. M. de Groot, H. Elnaggar, F. Frati, R.-p. Wang, M. U. Delgado-Jaime, M. van Veenendaal, J. Fernandez-Rodriguez, M. W. Haverkort, R. J. Green, G. van der Laan, Y. Kvashnin, A. Hariki, H. Ikeno, H. Ramanantoanina, C. Daul, B. Delley, M. Odelius, M. Lundberg, O. Kuhn, S. I. Bokarev, E. Shirley, J. Vinson, K. Gilmore, M. Stener, G. Fronzoni, P. Decleva, P. Kruger, M. Retaigan, Y. Joly, C. Vorwerk, C. Draxl, J. Rehr, and A. Tanaka, *Journal of Electron Spectroscopy and Related Phenomena* **249**, 147061 (2021).

[13] G. van der Laan, J. Zaanen, G. A. Sawatzky, R. Karnatak, and J.-M. Esteve, *Phys. Rev. B* **33**, 4253 (1986).
